# Supplementary material for: Linguistics-aware Masked Image Modeling for Self-supervised Scene Text Recognition
Source: arXiv:2503.18746 source file (2025-03-24)
Supplement: Supplementary file 1 [file suppl.tex]

\clearpage
\setcounter{page}{1}

\maketitlesupplementary

%%%%%%%%%%%%%%%%%%%%%%%%%%%%%
\section{Code}
We provide the code for the pre-training and fine-tuning phases of our method in the accompanying zip file to demonstrate reproducibility.
In addition, we also include code for extracting cropped text regions from crawled images using PaddleOCR~\footnote{\raggedright\url{https://github.com/PaddlePaddle/PaddleOCR}}.

%%%%%%%%%%%%%%%%%%%%%%%%%%%%%%%%%%%%%%
\section{Dataset}
\label{sec:rationale}
We provide a detailed introduction to each dataset used during pre-training, fine-tuning, and evaluation phases. 

\textbf{Pre-training Data.} The Union14M-U~\cite{union14m_sstr_iccv23} dataset consists of three subsets: Book32 with approximately 2.7 million images, CC with about 5.6 million images, and OpenImages containing roughly 2.3 million images. 

For the Chinese dataset, we collected approximately 5 million images from the Web and utilized PaddleOCR to generate about 11 million cropped images based on specific filtering criteria. During the filtering stage, we excluded cropped areas smaller than 400 pixels and those with a confidence score below 0.9.

\textbf{Fine-tuning Data.} Union14M-L~\cite{union14m_sstr_iccv23} includes five subsets for fine-tuning: Challenging with 482,877 images, Easy with 2,076,161 images, Hard with 308,025 images, Medium with 145,525 images, and Normal with 218,154 images. The Chinese benchmark~\cite{chinese_benchmark_arxiv21} for fine-tuning comprises four subsets: Scene with 509,164 images, Web with 112,471 images, Document with 400,000 images, and Handwriting with 74,603 images.

\textbf{Benchmarks.} Among the six commonly used benchmarks, IIIT5K~\cite{iiit_5k_bmvc12} contains 3,000 images, IC13~\cite{ic13_icdar13} contains 1,015 images, SVT~\cite{svt_iccv11} contains 647 images, IC15~\cite{icdar15_icdar15} contains 2,077 images, SVTP~\cite{svtp_iccv13} contains 645 images, and CUTE~\cite{cute80_eswa14} contains 288 images. For the Union14M benchmark~\cite{union14m_sstr_iccv23}, the subsets are as follows: Curve with 2,426 images, Multi-oriented with 1,369 images, Artistic with 900 images, Contextless with 779 images, Salient with 1,585 images, Multi-words with 829 images, and General with 400,000 images. In the Chinese benchmark~\cite{chinese_benchmark_arxiv21}, Scene comprises 63,646 images, Web comprises 14,059 images, Document comprises 50,000 images, and Handwriting comprises 23,389 images.
\section{Additional Visualization}

We visualize the attention maps of traditional MIM and our LMIM on the Chinese dataset in~\cref{fig:attvis_cn}. The results reveal that the MIM method predominantly focuses on local regions, such as the specific Chinese characters corresponding to the query, whereas our LMIM places greater emphasis on the global context. Since the Chinese language relies heavily on linguistic information, this difference highlights the strength of our approach. Notably, the observed attention map patterns align with the quantitative experimental results, further demonstrating that our method effectively captures linguistic information.

\begin{figure*}
  \centering
  \includegraphics[width=2\columnwidth]{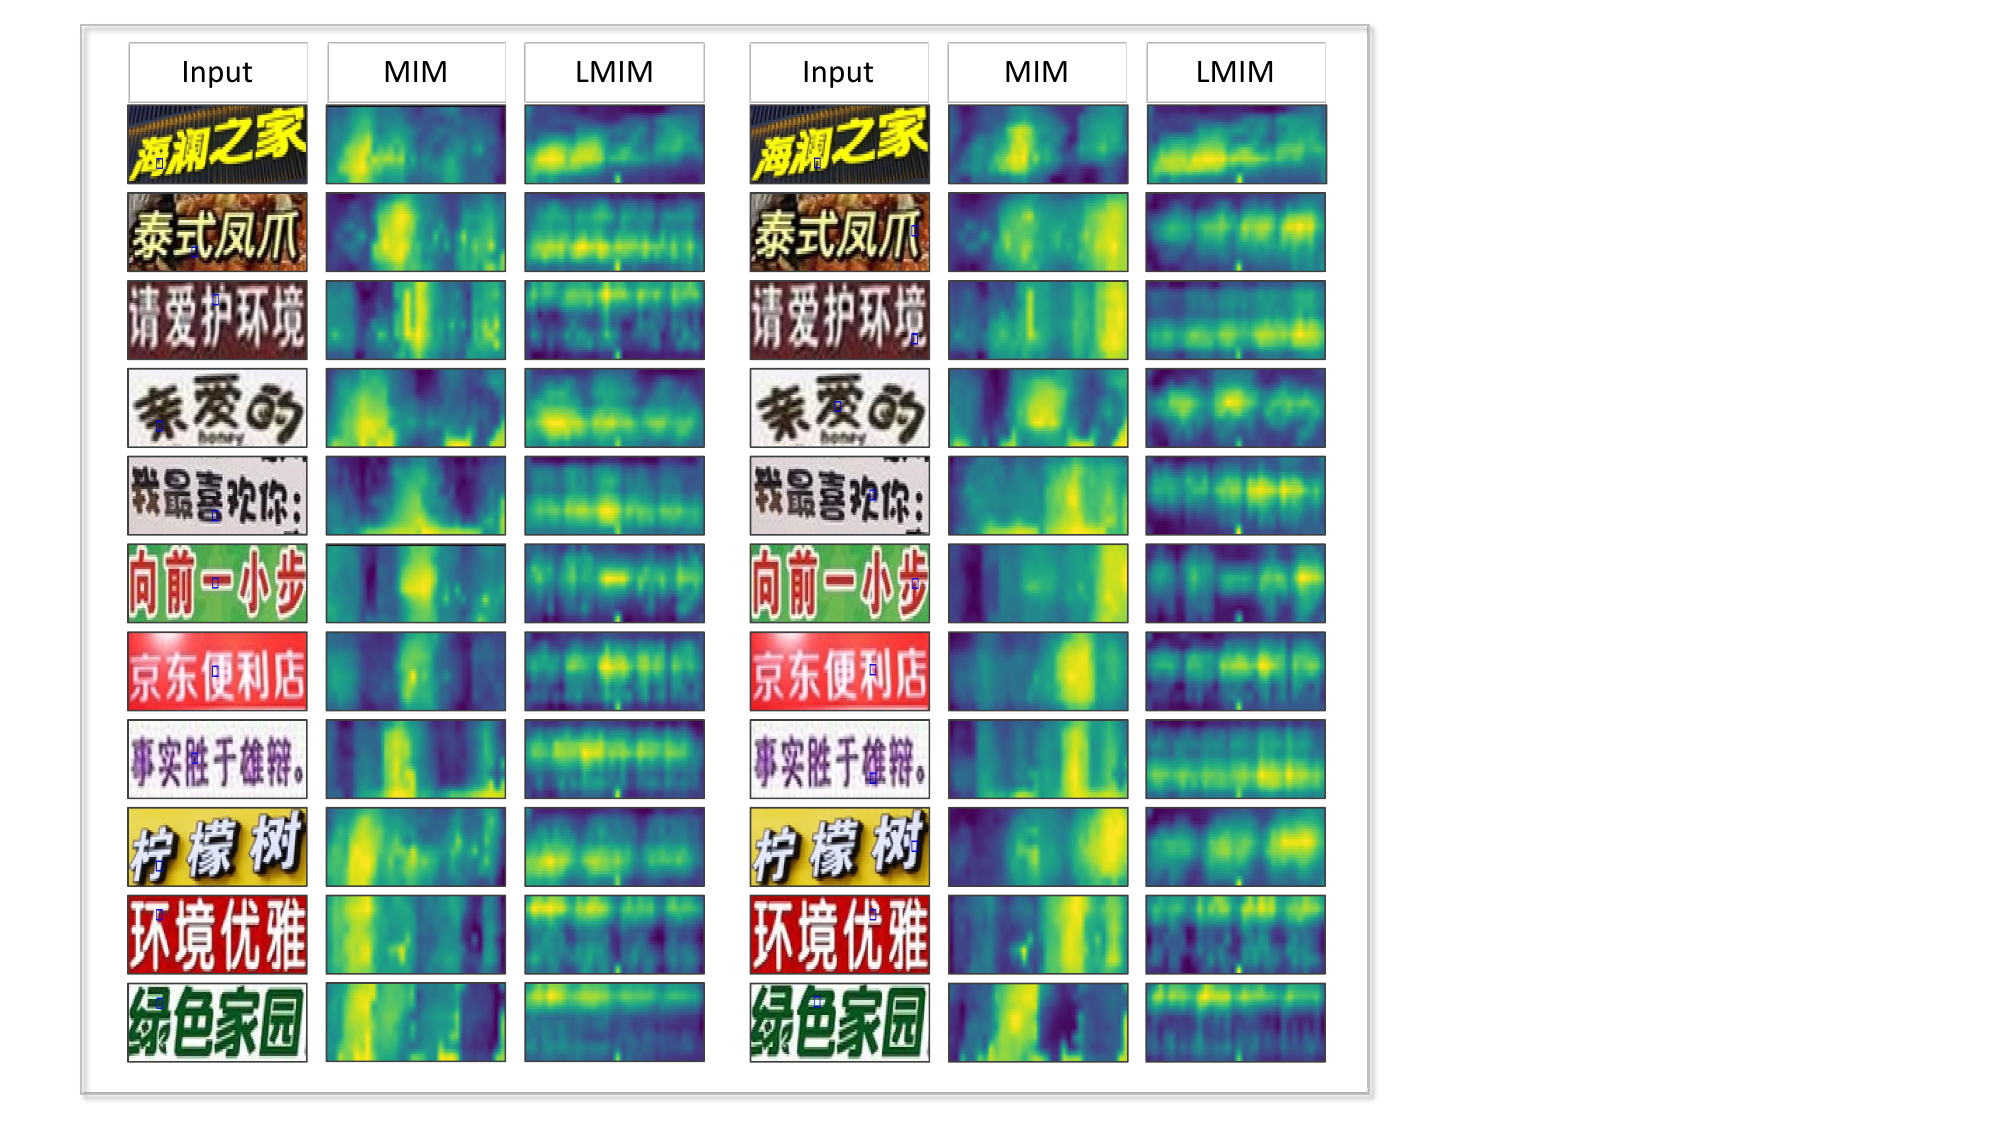}
  
    \caption[]{Visualization of attention maps on Chinese data. The blue box in the input image refers to the query.}
    \label{fig:attvis_cn}
\end{figure*}
